# Supplementary material for: MagicSeg: Open-World Segmentation Pretraining via Counterfactural Diffusion-Based Auto-Generation
Source: arXiv:2603.19575 source file (2026-03-20)
Supplement: Supplementary file 1 [file X_suppl.tex]

\clearpage
\setcounter{page}{1}
\maketitlesupplementary

\section{Text Generation Conditions}
Our conditions for ChatGPT to generate text prompts can be seen in Figure \ref{fig:prompt_app}.

\begin{figure*}[hb!]
    \centering
    \includegraphics[width=1.0 \linewidth]{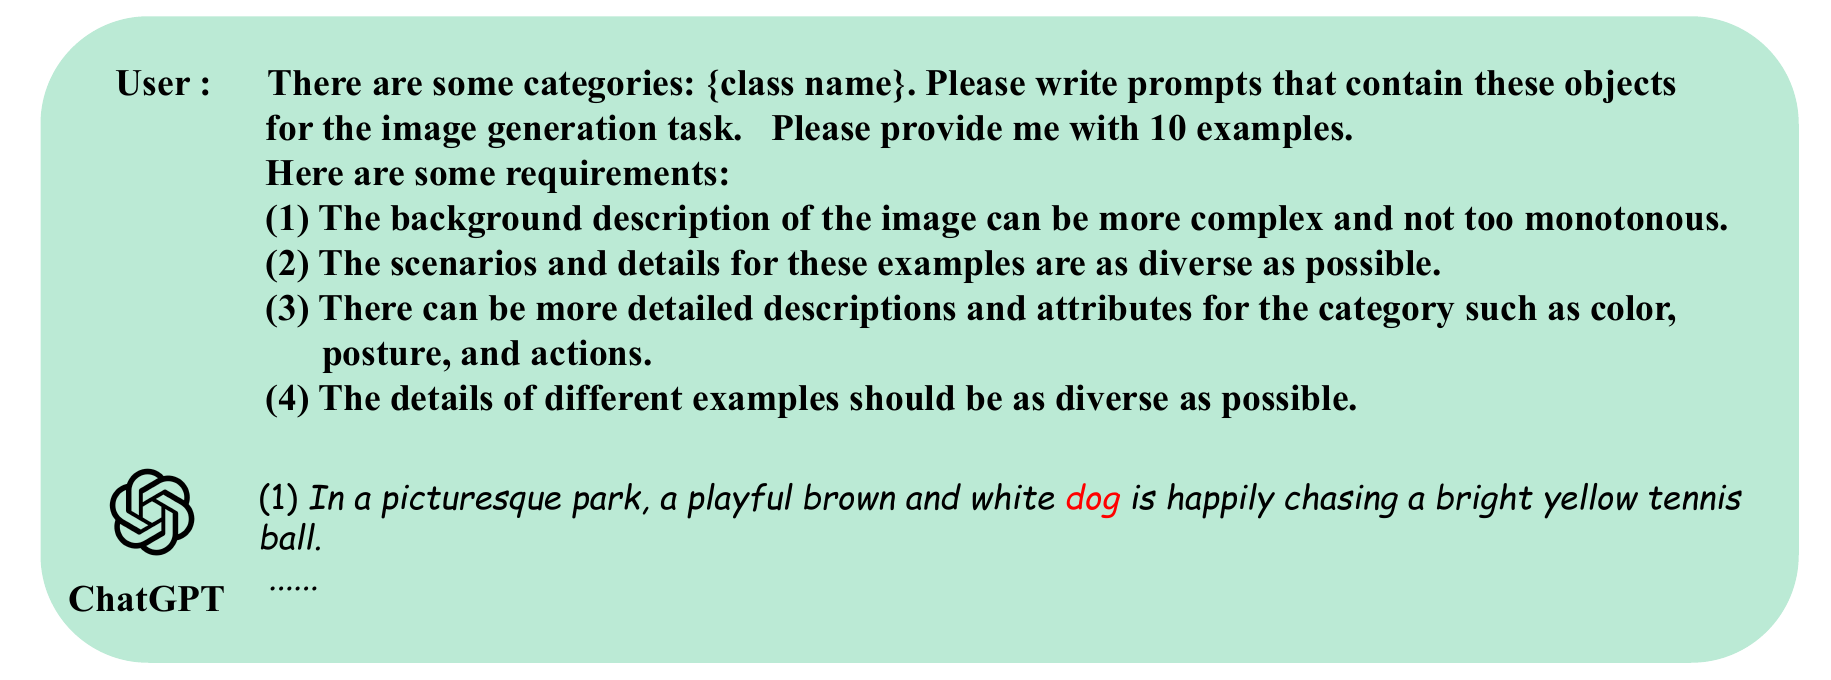}
    \caption{Text Prompt Generation Conditions for ChatGPT.}
    \label{fig:prompt_app}
\end{figure*}

\section{Dataset Visualization}
We show MagicSeg's dataset which contains texts, images, masks, and counterfactual images in Figure \ref{fig:data_app}.

\begin{figure*}[hb!]
    \centering
    \includegraphics[width=1.0 \linewidth]{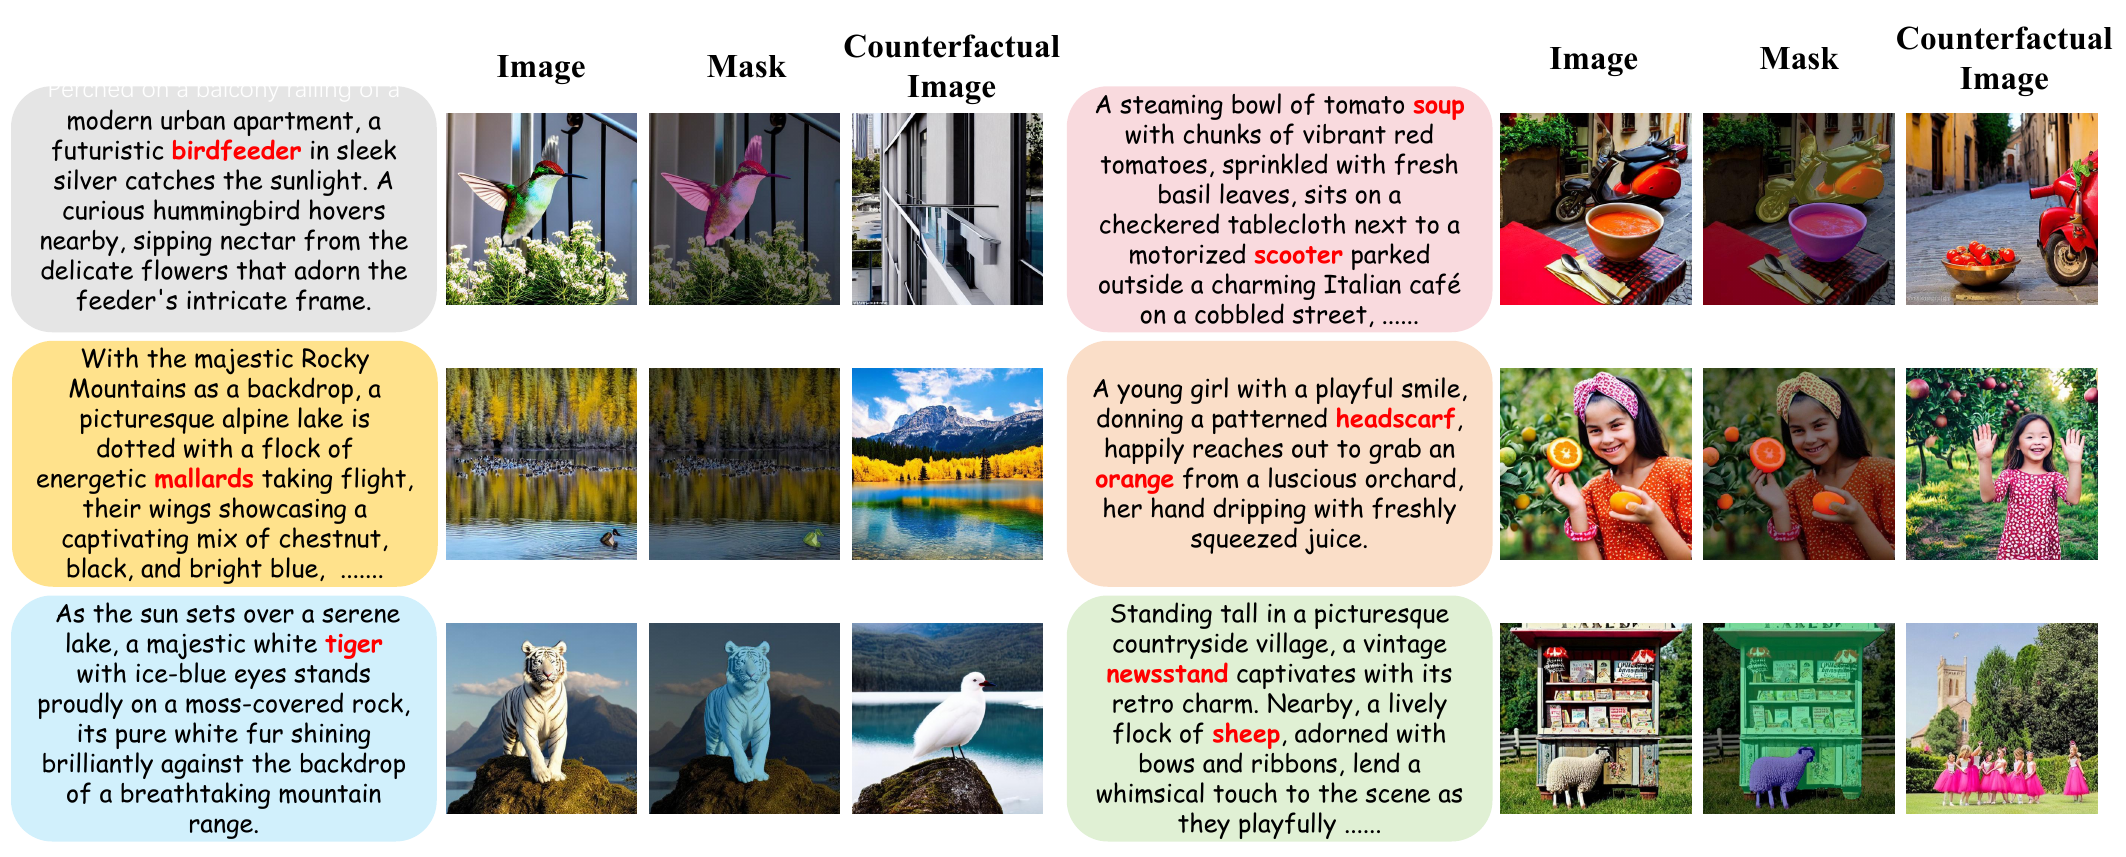}
    \caption{Visualization of MagicSeg's dataset.}
    \label{fig:data_app}
\end{figure*}

\section{Segmentation Results}
As shown in Figure \ref{fig:seg_appendix}, we show more semantic segmentation results on PASCAL VOC and COCO predicted by GroupViT and MagicSeg. It can be seen that, compared to GroupViT, MagicSeg has more advantages in fine-grained recognition.

\begin{figure*}[ht!]
% \vspace{-0.5em}
    \centering
    \subfloat[PASCAL VOC]{\includegraphics[width=0.45\linewidth]{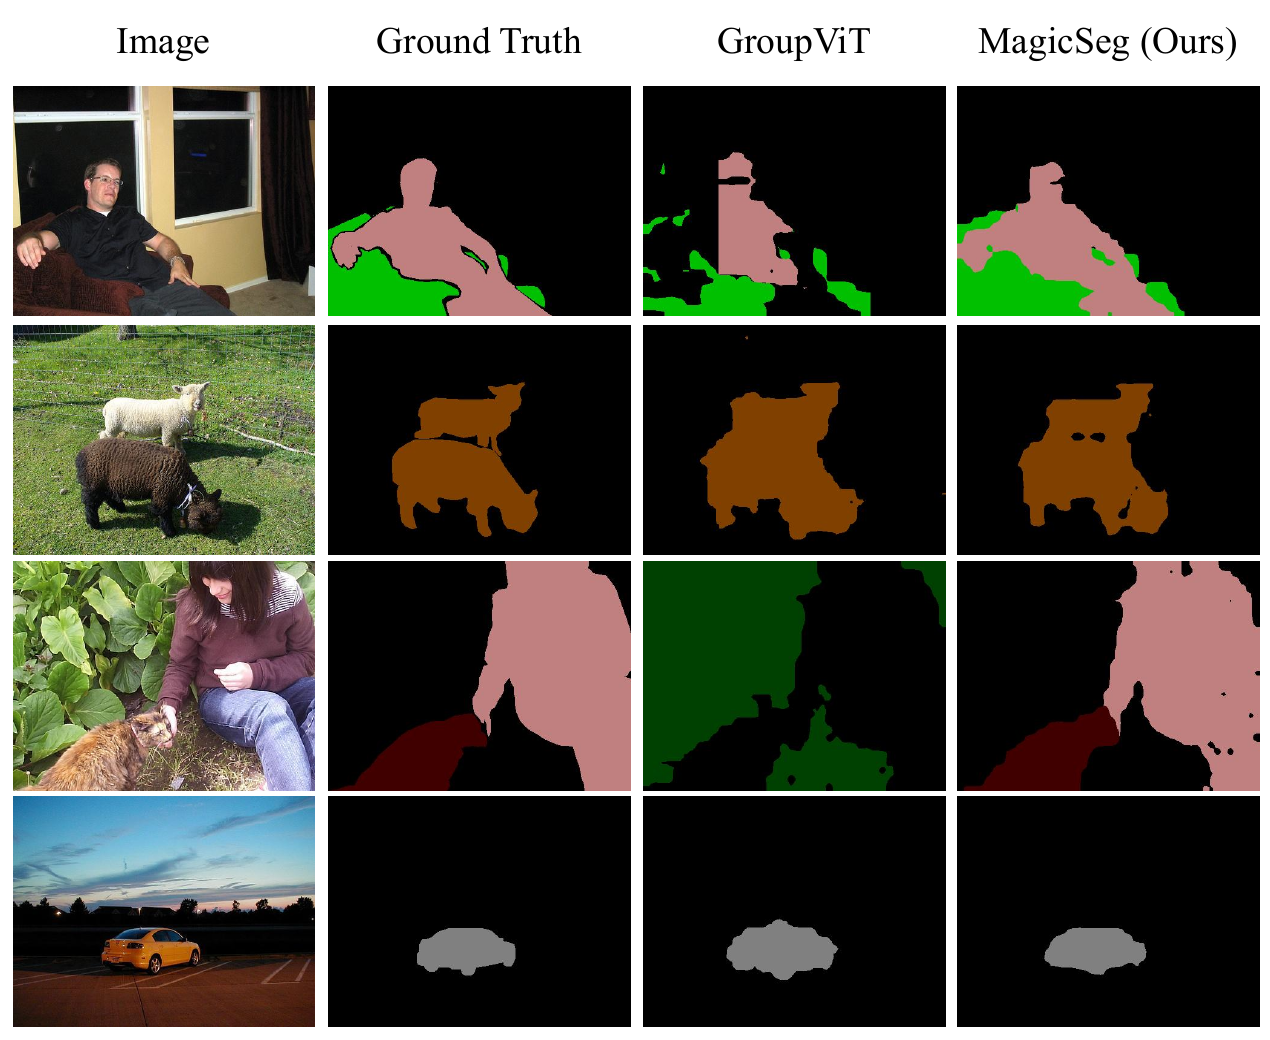}}
    \hspace{0.5em}
    \subfloat[COCO] {\includegraphics[width=0.45\linewidth]{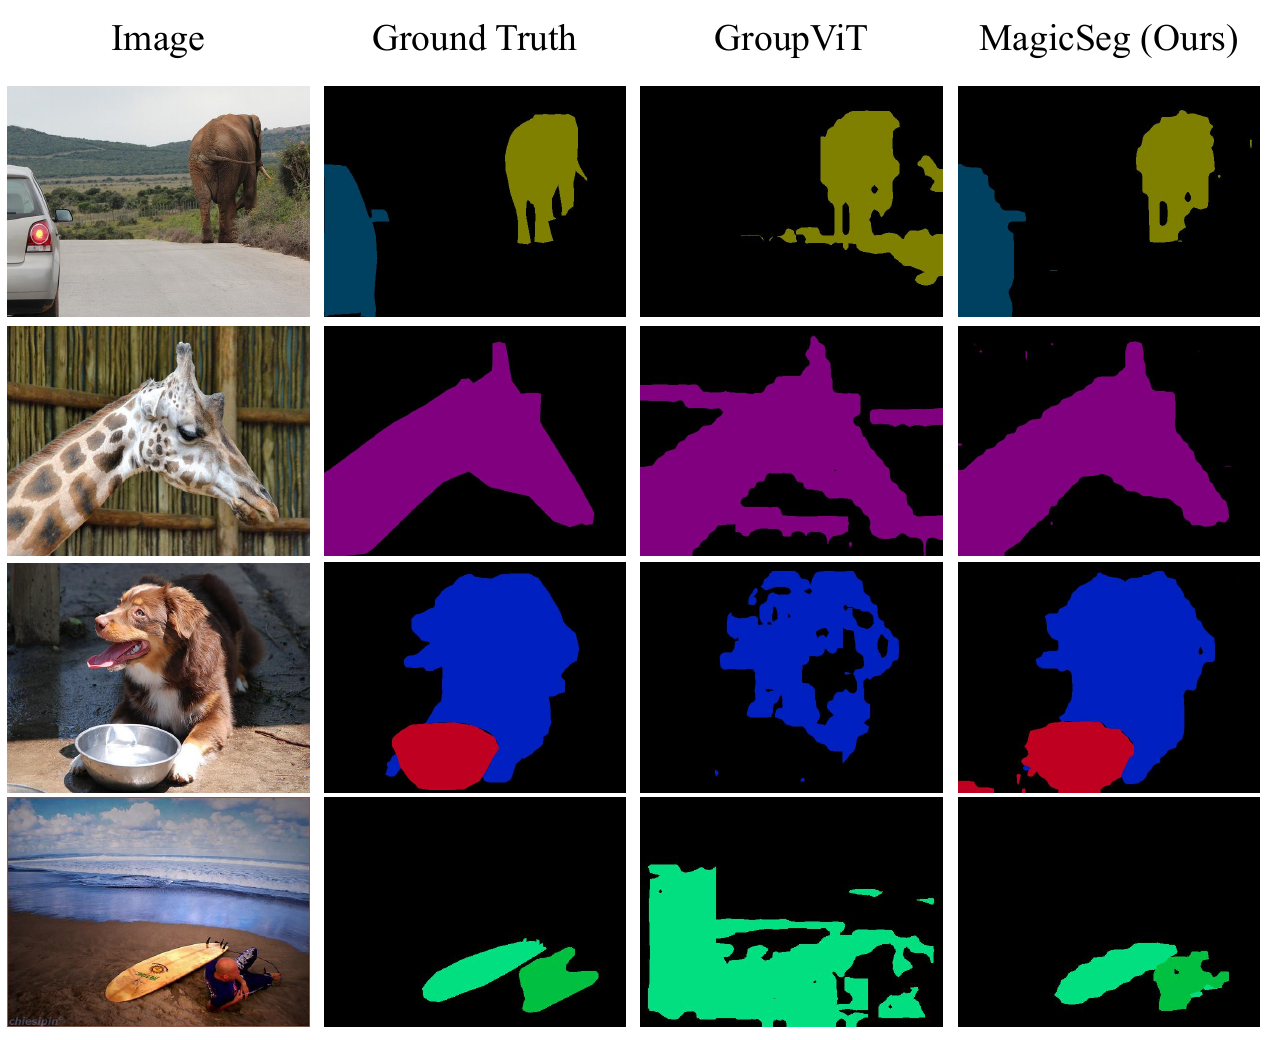} }
    \vspace{-1em}
    \caption{
        More semantic segmentation results on PASCAL VOC and COCO.
    }
    \label{fig:seg_appendix}
    \vspace{-1.2em}
\end{figure*}
